# Supplementary material for: RoBCtrl: Attacking GNN-Based Social Bot Detectors via Reinforced Manipulation of Bots Control Interaction
Source: arXiv:2510.16035 source file (2025-10-16)
Supplement: Supplementary file 1 [file 6-appendix.tex]

\clearpage
\section{Appendix}
\label{sec:append}

\subsection{\DiffBot Training and Bot Generation Algorithms}

\begin{algorithm}
\caption{\DiffBot Training}
\label{algorithm1}
\KwIn{All labelled users' feature $X$ and randomly initialized $\theta$.}
\Repeat{$\theta$ \rm{converged}}{
    Sample a batch of users' features $X_b\subset X$ \label{alg1:sample}\;
    \For {\rm{all} $x_0 \in X_b$ }{ \label{alg1:sample2}
    Sample $t\sim \mathcal{U}(1,T)$ or $t\sim p_t,\epsilon \sim \mathcal{N}(0,\boldsymbol{I})$ \;
    Compute $x_t$ given $x_0,t$ and $\epsilon$ via $q(x_t|x_0)$ in Eq.\ref{formula:qxt0} \;
    Compute $\mathcal{L}_t$ by Eq.\ref{formula:Lt} if $t>1$, otherwise by Eq.\ref{formula:l1} \; \label{alg1:loss_fuc}
    Calculate $\nabla_{\theta}\mathcal{L}_t$ to optimize $\theta$ \; \label{alg1:backpropagation}
    }
} 
\KwOut{Optimized $\theta$}
\end{algorithm}
Algorithm.\ref{algorithm1} summarizes the training process of \DiffBot. Firstly, repeat sample batch users' features from $X$ (Line \ref{alg1:sample}), then sample the time step $t$ and calculate the chosen loss function according to $t$ (Lines \ref{alg1:sample2}-\ref{alg1:loss_fuc}).  Finally, the gradient backpropagation optimization parameters are calculated (Line \ref{alg1:backpropagation}). The process is repeated until the parameters converge.

\begin{algorithm}
\caption{Bot Generation}
\label{algorithm2}
\KwIn{$\theta$, the sampled users' feature set $\mathcal{U}_b$, generated users set $\mathcal{U}_g$}
\For {$u\in\mathcal{U}_b$}{  \label{alg2:sample} 
    Set $x_0=x_u$ and sample $\epsilon \sim \mathcal{N}(0,\boldsymbol{I})$ \; \label{alg2:setx0}
    Compute $x_{T'}$ via $x_0,T',\epsilon$ via Eq.\ref{formula:qxt0}, and set $\hat{x}_T=x_{T'}$\; \label{alg2:XT}
    \For {$t=T,\cdots$,1}{ \label{alg2:denoise}
        $\hat{x}_{t-1}=\mu_\theta(\hat{x}_t,t)$ calculated from $\hat{x}_t$ and $\hat{x}_\theta(\cdot)$ via Eq.\ref{formula:mutheta} \;
    } \label{alg2:denoise_end}
    Add $\hat{x}_0$ to $\mathcal{U}_g$\; \label{alg2:add_user}
} 
\KwOut{Generated $\mathcal{U}_g$}
\end{algorithm}
Algorithm.\ref{algorithm2} outlines the process of bot generation using the \DiffBot model. Firstly, a user $x_u$ is selected to be replicated (Line \ref{alg2:sample}), and it is set as the initial user feature for the forward propagation of the diffusion model (Line \ref{alg2:setx0}). The final noisy feature $x_{T'}$ is computed directly based on the predetermined final time step $T'$, as specified by Eq.\ref{formula:qxt0} (Line \ref{alg2:XT}). Subsequently, the noisy feature $x_{T'}$ is repeatedly denoised to generate replicated vectors $\hat{x}_0$ (Lines \ref{alg2:denoise}-\ref{alg2:denoise_end}), which are added to the generated user set $\mathcal{U}_g$ (Line \ref{alg2:add_user}). This process is iterated until the generated users match the predetermined number.

\subsection{The Social Bot Attack Algorithm}
\begin{algorithm}
\caption{\RoBCtrl}
\label{algorithm3}
\KwIn{Social graph $\mathcal{G}$, pre-trained surrogate model $f_{\theta}*$, action aggregation probability $\mathcal{P}$, memories $\mathcal{M}$}
\DiffBot training defined in Algorithm.\ref{algorithm1}\; \label{alg3:traindiff}
Evolved bot generation defined in Algorithm.\ref{algorithm2}\; \label{alg3:genbots}
Add evolved bots' features to $\mathcal{G}$ \; \label{alg3:addbots}
Initialize $N$ RL agents \;  \label{alg3:initialagents}
\For{$t=0,1,\ldots,T$}{
    Query the index $i$ of $v_t$\; \label{alg3:choosev}
    $s_t=[\rm{pool}(e(\mathcal{G}_t)),e(\mathcal{G}_t)_{[i]}]$ \; \label{alg3:calstate}
    $a_t'=(a_t^1,a_t^2,a_t^3)$ via Eq.\ref{eq:PI}\;  \label{alg3:calaction}
    Choose action $a_t$ from $a_t'$ according $\mathcal{P}$ \;   \label{alg3:chooseaction}
    Add edge $(i,a_t)$ to obtain $\mathcal{G}_t'$\; \label{alg3:addedge}
    Obtain $R((\mathcal{G}_t,f_{\theta*})_v)$ via Eq.\ref{eq:reward} \; \label{alg3:calreward}
    \For{$j=1,2,\ldots,N$}{
        Store the $T^j_t=(s_t,a^j_t,s_{t+1}, R((\mathcal{G}_t,f_{\theta*})_v))$ into $\mathcal{M}_j$ \; \label{alg3:storememory}
    }
    \For{$j=1,2,\ldots,N$}{
        Optimize $\pi^j$ via Eq.\ref{eq:rl_optimize}\; \label{alg3:optiagent}
    }
}
Attack $\mathcal{G}$ via agents to obtain $\mathcal{G}'$\;  \label{alg3:attack}
\KwOut{Perturbed Social Graph $\mathcal{G}'$}
\end{algorithm}
Algorithm \ref{algorithm3} describes the attack process of \RoBCtrl on a Graph Neural Network detector for social bot attacks. Firstly, the parameters of the \DiffBot model are trained (Line \ref{alg3:traindiff}), and then the model is used to generate evolved bots (Line \ref{alg3:genbots}). The nodes and features of these evolved bots are added to graph $\mathcal{G}$ (Line \ref{alg3:addbots}). Multi-agent reinforcement learning parameters are initialized (Line \ref{alg3:initialagents}). The i-th node is identified (Line \ref{alg3:choosev}), and calculate the environmental state value of the node (Line \ref{alg3:calstate}). Reinforcement learning agents are used to select an action (Lines \ref{alg3:calaction}-\ref{alg3:chooseaction}), and then the edge represented by that action is added to the poisoned graph $\mathcal{G}_t'$ (Line \ref{alg3:addedge}). Then compute the reward value (Line \ref{alg3:calreward}). And store the state transition entries into memory (Line \ref{alg3:storememory}), and optimize the parameters of the agents' policy networks (Line \ref{alg3:optiagent}). This process is repeated until the reinforcement learning agent parameters converge. Finally, the poisoned graph $\mathcal{G}'$ is obtained by utilizing the reinforcement learning agent to attack graph $\mathcal{G}$ (Line \ref{alg3:attack}).

% \begin{figure*}[t]
% % \setlength{\abovecaptionskip}{0.15cm}
% \setlength{\belowcaptionskip}{-0.35cm}
%     \centering
%     \includegraphics[width=0.99\linewidth]{assets/Visual.png}
%     \caption{. } 
%     \Description{The visualization result.}
%     \label{fig:framework}
% \end{figure*}
% % \begin{figure*}[t]
